# Supplementary material for: Towards Reliable Latent Knowledge Estimation in LLMs: Zero-Prompt Many-Shot Based Factual Knowledge Extraction
Source: arXiv:2404.12957 source file (2024-12-17)
Supplement: Supplementary file 1 [file old_all_results.tex]

\section{Detailed results of the evaluation of all models}

Table \ref{table:all_results} displays Probability Mass and Precision results for various models.

\label{appendix: all_results}
\begin{table}[h]
    \centering
    \caption{Evaluation Results for all Models}
    \label{table:all_results}
    \begin{tabular}{l c c c}
        \toprule
        Model & Prob Mass & Precision\\
        \midrule
        Pythia-70m  &0.0132 &0.0242 \\
        Pythia-160m   &0.0115 &0.0233 \\
        Pythia-410m  &0.0124  &0.0248 \\
        Pythia-1b  &0.0133  &0.0248\\
        Pythia-1.4b  &0.0136  &0.0268 \\
        Pythia-2.8b   &0.0125 &0.0190\\
        Pythia-6.9b  &0.0130 &0.0216 \\
        Pythia-12b  &0.0131 &0.0228 \\
        LLaMA-7b    &0.0166 &0.0291 \\
        LLaMA-13b   &0.0208  &0.0360\\
        LLaMA-33b   &0.0276  &0.0469 \\
        LLaMA-65b     &0.0281  &0.0518 \\
        LLaMA-2-7b   &0.0197 &0.0232 \\
        LLaMA-2-13b &0.0249 &0.0357 \\
        LLaMA-2-70b &0.0379 &0.0616 \\
        LLaMA-2-7b-chat &0.0175 &0.0259 \\
        LLaMA-2-13b-chat &0.0206 &0.0263 \\
        LLaMA-2-70b-chat &0.0351 &0.0460 \\
        
        \bottomrule
    \end{tabular}
\end{table}

% \begin{figure}[ht]
%     \centering
%     \noindent\begin{minipage}{\textwidth}
%         \centering
%         \subfloat[Entropy]{
%         \includegraphics[width=.3\linewidth]{plots/pythia-Entropy.pdf}}
%         \subfloat[PMF]{
%         \includegraphics[width=.3\linewidth]{plots/pythia-PMF.pdf}}
%         \subfloat[Precision]{
%         \includegraphics[width=.3\linewidth]{plots/pythia-Precision.pdf}}
%     \end{minipage}
%     \caption{Average results of the 3 metrics for Pythia models}
%     \label{fig:pythia_evaluation}
% \end{figure}


% \begin{figure}[ht]
%     \centering
%     \noindent\begin{minipage}{\textwidth}
%         \centering
%         \includegraphics[width=.3\linewidth]{plots/llama-Entropy.pdf}
%         \includegraphics[width=.3\linewidth]{plots/llama-PMF.pdf}
%         \includegraphics[width=.3\linewidth]{plots/llama-Precision.pdf}
%     \end{minipage}

%     \caption{Average results of the 3 metrics for LLaMA models}
%     \label{fig:LLaMA_evaluation}
% \end{figure}
