# Supplementary material for: Towards Reliable Latent Knowledge Estimation in LLMs: Zero-Prompt Many-Shot Based Factual Knowledge Extraction
Source: arXiv:2404.12957 source file (2024-12-17)
Supplement: Supplementary file 2 [file old_diff_prompts.tex]

\section{Results for different prompts}
\label{app:diff_prompts}

\begin{table}[]
    \centering
    \caption{Different Prompt Templates with Examples}
    \label{table:different_prompts}
\begin{tabular}{ccc}
\hline
\textbf{Key}     & \textbf{Template}                     & \textbf{Example}                     \\ \hline
entity\_rel      & \{entity\} \{relationship\}           & Albert Einstein birth year           \\
entity\_rel\_is  & \{entity\} \{relationship\} is        & Albert Einstein birth year is        \\
entitys\_rel\_is & \{entity\}'s \{relationship\} is      & Albert Einstein's birth year is      \\
rel\_of\_entity  & The \{relationship\} of \{entity\} is & The birth year of Albert Einstein is \\
crafted          & \{entity\} was born in the year       & Albert Einstein was born in the year \\ \hline
\end{tabular}
\end{table}

\begin{figure}[ht]
    \centering
    \noindent\begin{minipage}{\textwidth}
        \centering
        % \subfloat[Entropy]{
        % \includegraphics[width=.3\linewidth]{plots/diff_prompts_entropy.pdf}}
        \subfloat[PMF]{
        \includegraphics[width=.5\linewidth]{plots/diff_prompts_pmf.pdf}}
        \subfloat[Precision]{
        \includegraphics[width=.5\linewidth]{plots/diff_prompts_precision.pdf}}
    \end{minipage}
    \caption{Average results of the 3 metrics for Different Prompts}
    \label{fig:diff_prompts}
\end{figure}

We try out 5 different prompts templates described in Table \ref{table:different_prompts}. We  report the aggregate results for each of the prompts in Fig. \ref{fig:diff_prompts}.

All prompts yield similar results, and considering relative probabilities eliminates the need for prompts to generate the correct answer as output.
