# Supplementary material for: Towards Reliable Latent Knowledge Estimation in LLMs: Zero-Prompt Many-Shot Based Factual Knowledge Extraction
Source: arXiv:2404.12957 source file (2024-12-17)
Supplement: Supplementary file 3 [file old_manual_prompts.tex]

\clearpage
\section{Traditional prompt-based estimation}
\label{appendix:maunual_prompts}

This appendix details the specific parameters used for prompt generation. Table~\ref{table:model-accuracy-comparison}, in the main paper, presents the accuracy, \( A(r) \), for four different models, comparing the results obtained from manually designed tests and our LKEs.

For this experiment, we considered two types of prompts to directly checking for the top answer (temperature = 0, top-k = 1): zero shot prompting and few shot prompt.

For Zero Shot prompting, the structure is as follows:

\textbf{Zero Shot:}
\begin{verbatim}
Answer the following question in as few words as possible. 
In what year was {subject} born? Answer:
\end{verbatim}

For Few Shot prompting, the format is:

\textbf{Few Shot:}
\begin{verbatim}
 "Answer the following questions in as few words as possible. 
                          Question: In which year was Einstein born?
                          Answer: 1879
                          Question: In which year was Thomas Alva Edison born?
                          Answer: 1847
                          Question: In which year was {subjct} born?
                          Answer: ",
\end{verbatim}

where \({subject}\) represents the name of Nobel laureates. The responses are evaluated based on the top 1 generated answer.
